# Supplementary material for: Multivariate Rational Approximation
Source: arXiv:1912.02272 source file (2019-12-03)
Supplement: Supplementary file 1 [file appendixperformance.tex]

\section{Discussion of computational performance}

This bit is really about comparing the monomial basis (MNB) approaches with their
orthonormal (ONB) counterparts.

For MNB-based calculations, the basis is always known, as is the recurrence
relation needed to solve and evaluate for rational and polynomial
approximations.  ONB-based calculations, unsurprisingly, require the explicit
knowledge of the recursion matrix, $R$, that stores the projections required to
evaluate polynomials in the ONB.

We obtain $R$ using the Stieltjes procedure. The computational expense of the
latter strongly depends on the dimension of the parameter space and the highest
order polynomials ($M$) to be used for the basis. See \cref{fig:onbcalc}.
For very general applications with many different rational approximations,
allowing for different ONB for each object, the computational expense
quickly escalates.

The additional memory footprint in the ONB approach compared to MNB comes from
the storage of the $Mdof\times Mdof$ recursion matrix which can be substantial
for large enough dimension and $M$. For example, holding 1000 recurrence
matrices for a 7-dimensional problem with $M=5$ requires 5GB or memory.
If the ONB and therefore $R$ are the same for all parametrisations used
in an application, a single ONB and $R$ can be used.

The computational cost of evaluating the recurrence in the ONB is generally
larger than that of the MNB. For small enough problems the cost difference
is negligible. For e.g. a 5-dimensional parameter spaces with max polynomial
order 6 we find the ONB recurrence to be 4\dots5 times more expensive than
the MNB equivalent (See \cref{fig:recurcalc}, blue lines).

\begin{figure}
    \centering
    \includegraphics[width=.68\textwidth]{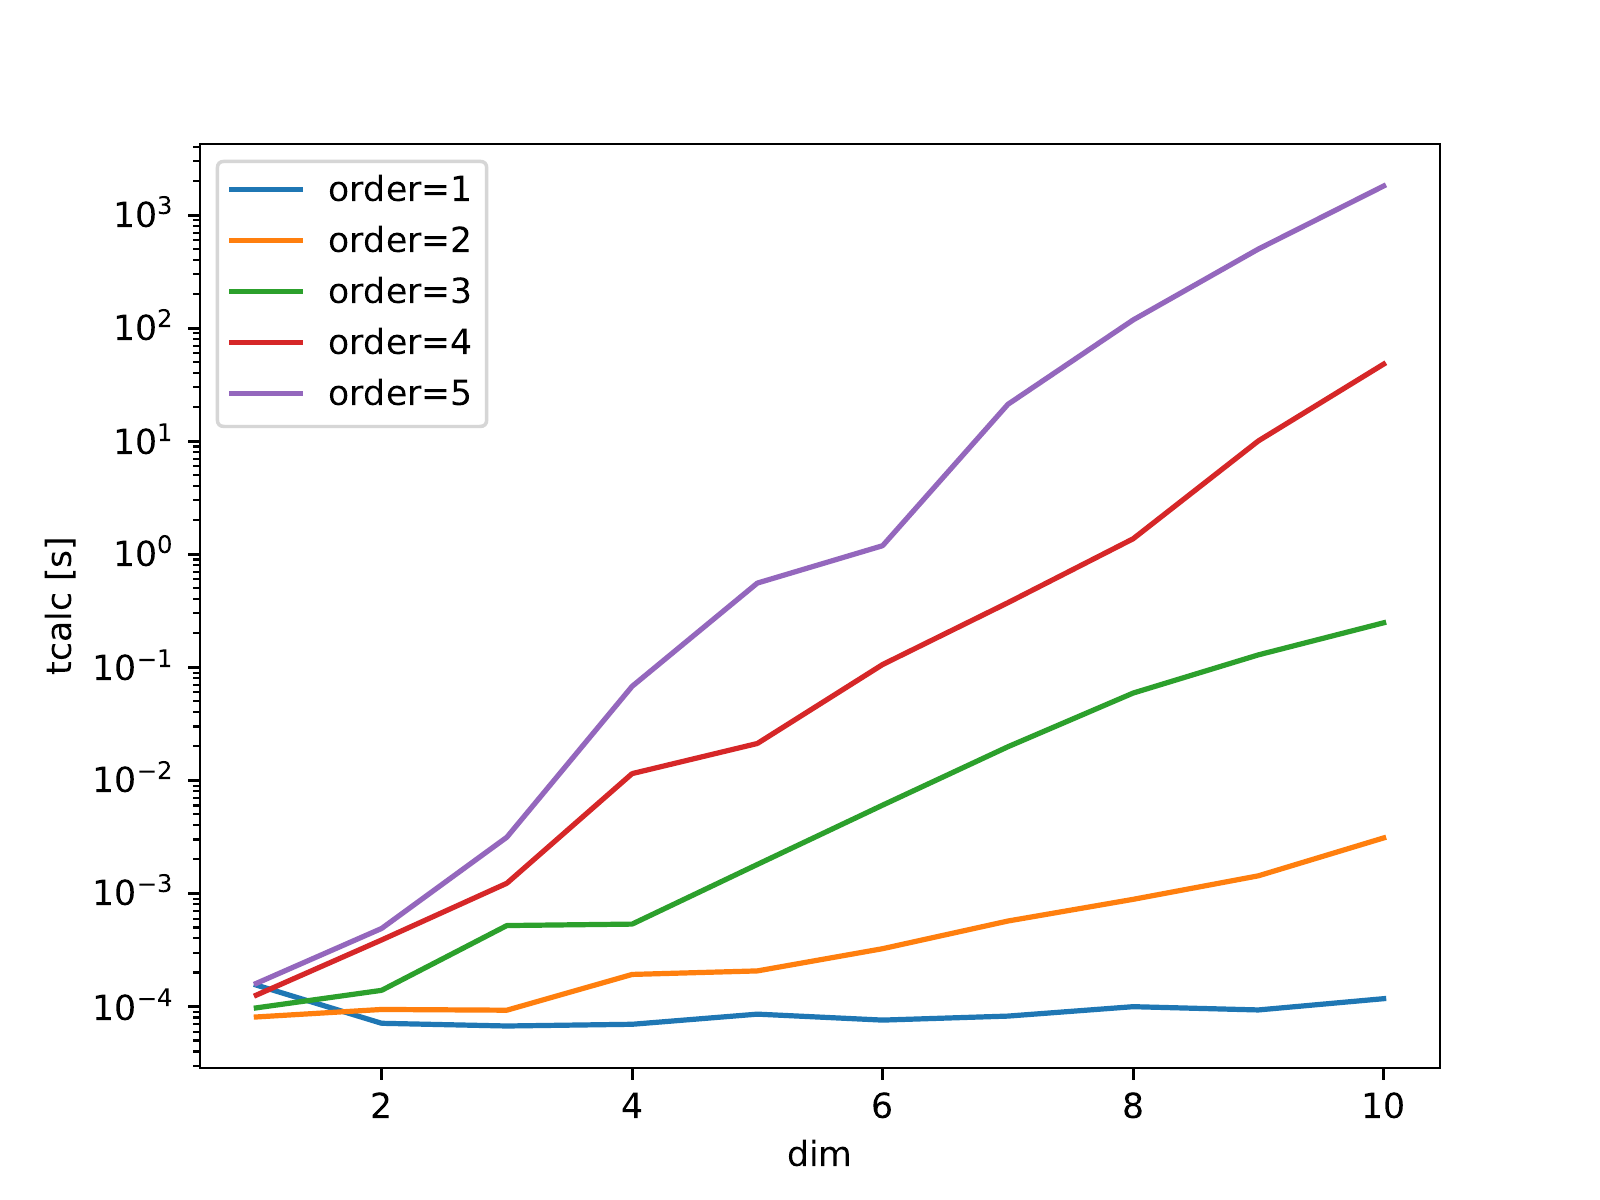}
    \caption{Computational expense of Stieltjes process as function of the dimensionality of the problem for different highest polynomial orders ($M$) to be used for the ONB. The datasets used for construction require $N_{points}=2 N_\text{min}(dim, M)$  }
    \label{fig:onbcalc}
\end{figure}

\begin{figure}
    \centering
    \includegraphics[width=.68\textwidth]{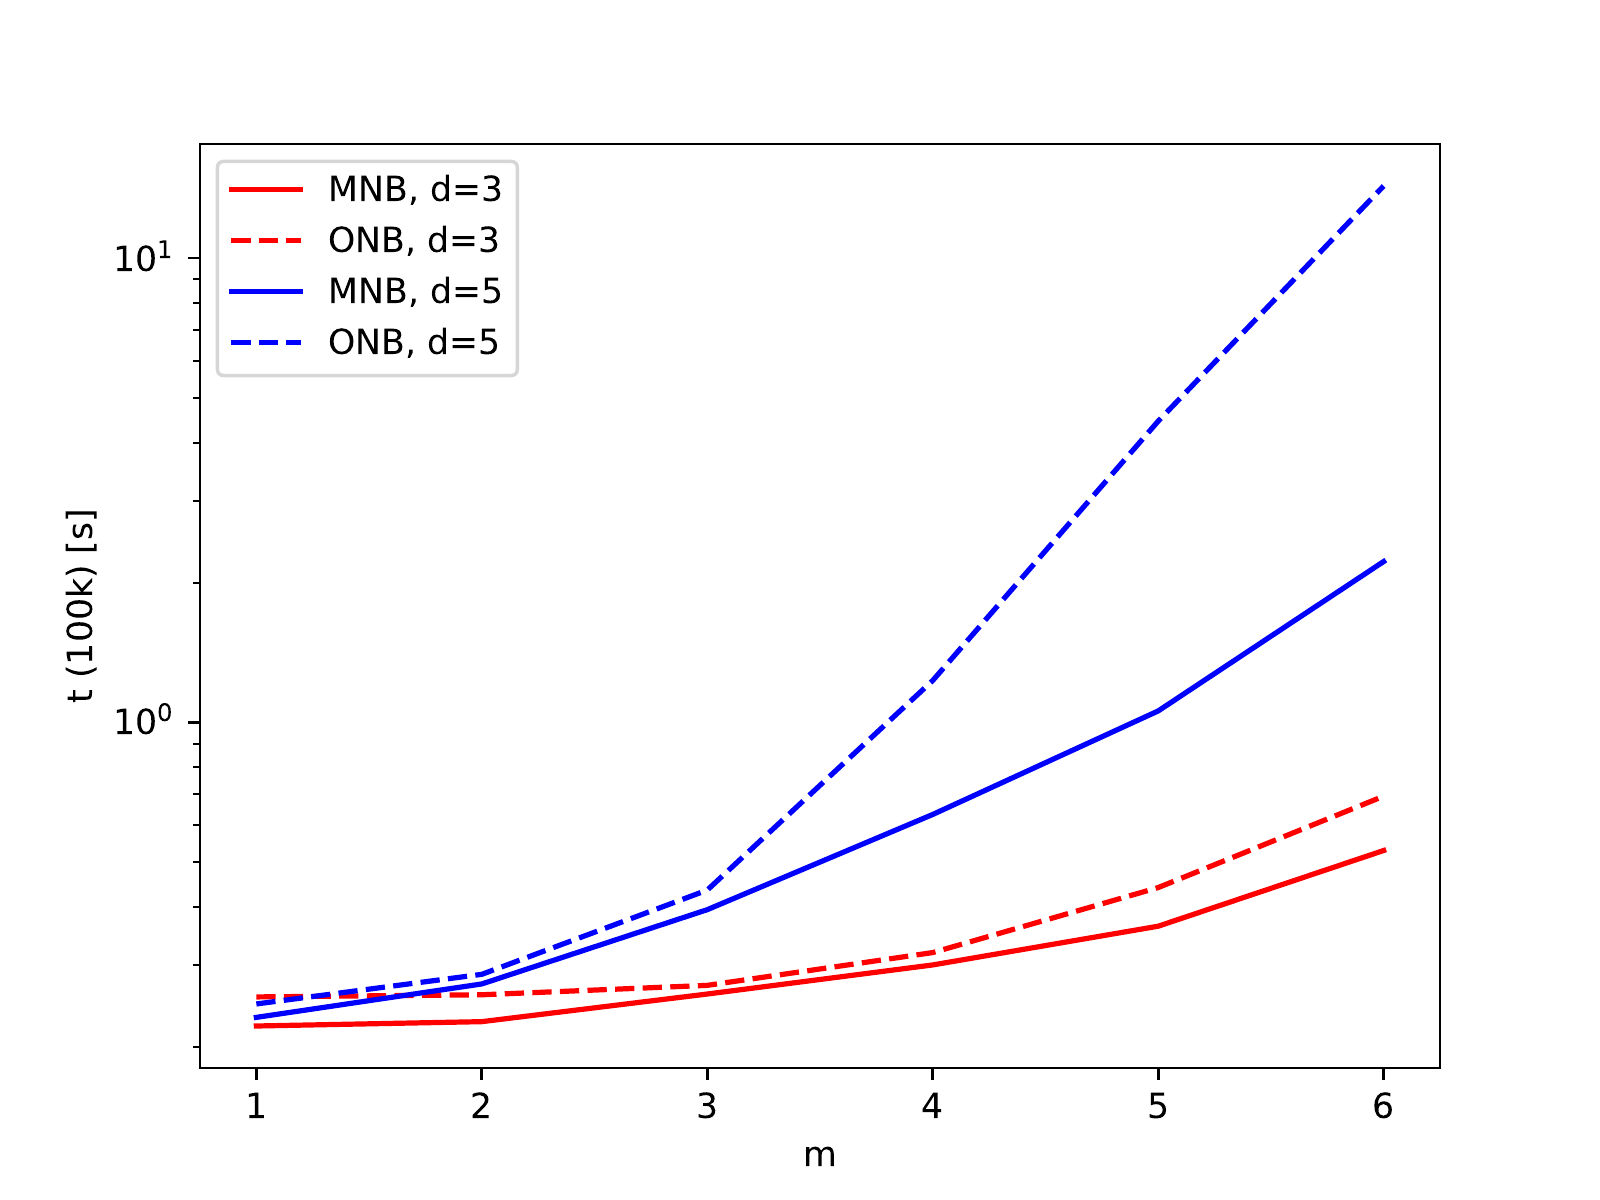}
    \caption{Computational cost of evaluating 100k recurrences in the ONB and MNB basis as function of the dimension of the problem for different max orders of polynomials.}
    \label{fig:recurcalc}
\end{figure}
