# Supplementary material for: Multivariate Rational Approximation
Source: arXiv:1912.02272 source file (2019-12-03)
Supplement: Supplementary file 2 [file apps_sm.tex]

\clearpage
\section{Rational Approximation for HEP Experiment}\label{SEC:HEP}
Physics simulation programs are used to make predictions of known or
proposed phenomenon that can be compared to experiments.
Typically, the physics models inside the simulation contain a large number of parameters.
Some of these have a fundamental physical meaning, such as masses and
coupling strengths.    Others are purely pragmatic and compound imperfect knowledge about certain aspects of the model.  Both types of parameters are needed to make accurate predictions.

A typical problem in particle physics is to infer 
%\emph{unobservable} 
values, or ranges of values, for the model parameters by comparing experimentally observed data with
equivalent quantities obtained from simulations of physics processes.
In our example, the simulation predicts how postulated dark matter particles
interact with a Xenon-based detector in a process called ``direct
detection''.   In practice, the simulation predicts a number of signal
counts in the detector with certain characteristics.     
If the characteristic is a continuous variable, it is sometimes
divided up into a finite number of bins $b$.
The signal
model is specified by three parameters $p = \{m_\chi, c_{+}, c_{\pi}\}$,
where $m_\chi$ is the mass of the dark matter candidate particle and
$c_{+}, c_{\pi}$ are coupling strengths for the interaction of the
dark matter with the ordinary matter in the detector.   The case $c_+
= c_\pi = 0$ corresponds to no dark matter signal.   Even in the
absence of a signal, counts are observed in the detector from backgrounds.
The number of counts in a given bin $b$ is expected to follow a
Poisson distribution with a mean value determined from the simulation
assuming no signal.   After data $d$ has been collected, an analysis is
performed to determine which values of $p$ are compatible or excluded.   The
statistic called Likelihood, $\mathcal{L}(p|d)$, is constructed and
maximized to answer
this question:
\begin{equation}\label{eq:alikelihood}
    \mathcal{L}(p|d) = \prod\limits_b \frac{N_b(p) d_b e^{N_b(p)}}{\Gamma(d_b+1)},
\end{equation}
where the product runs over all bins $b$, the numbers $d_b$ are
the experimentally measured quantities for each bin, and  $N_b(p)$ 
is the number of total counts in the bin $b$ predicted by the
parameters $p$, which range over a set of $k$ individual values $p^{(k)}$.

The calculation of $N_b(p^{(k)})$ is computationally expensive and can
only be performed at a finite number of points $p^{(k)}$.
Fortunately, the predictions are smooth and can be represented by a
surrogate function $r_b(p)$ constructed from a finite number of
calculations $N_b(p^{(k)})$.   Here, we demonstrate the utility of the
rational approximation methods in performing an accurate analysis of
the data in comparison to brute force and other approximation methods.   
Instead of maximizing the  likelihood in \cref{eq:likelihood}, we maximize an approximate likelihood:
\begin{equation}\label{eq:alikelihood-app}
    \mathcal{L}(x|d) \approx \mathcal{\tilde{L}}(x|d) = \prod\limits_b \frac{r_b(x) d_b e^{r_b(x)}}{\Gamma(d_b+1)}.
\end{equation}
The maximization of the likelihood itself is performed using 
the numerical tool MultiNest~\cite{Feroz:2008xx,Feroz:2013hea,pymultinest}.
 The data are simulated using a specific framework
of the generalized spin-independent response to dark matter in direct detection
experiments~\cite{Hoferichter:2016nvd}.
The $d_b$ used in
\cref{eq:likelihood,eq:likelihood-app} are 
 $d_b$ = \{ 70.4 , 26.7 , 9.8 , 3.4 , 1.0 , 0.2 \} for $b=6$ bins.
Note that we fit a separate rational approximation for each bin $b$.

% \begin{figure}[htb!]
%     \centering
%     \includegraphics[width=.68\textwidth]{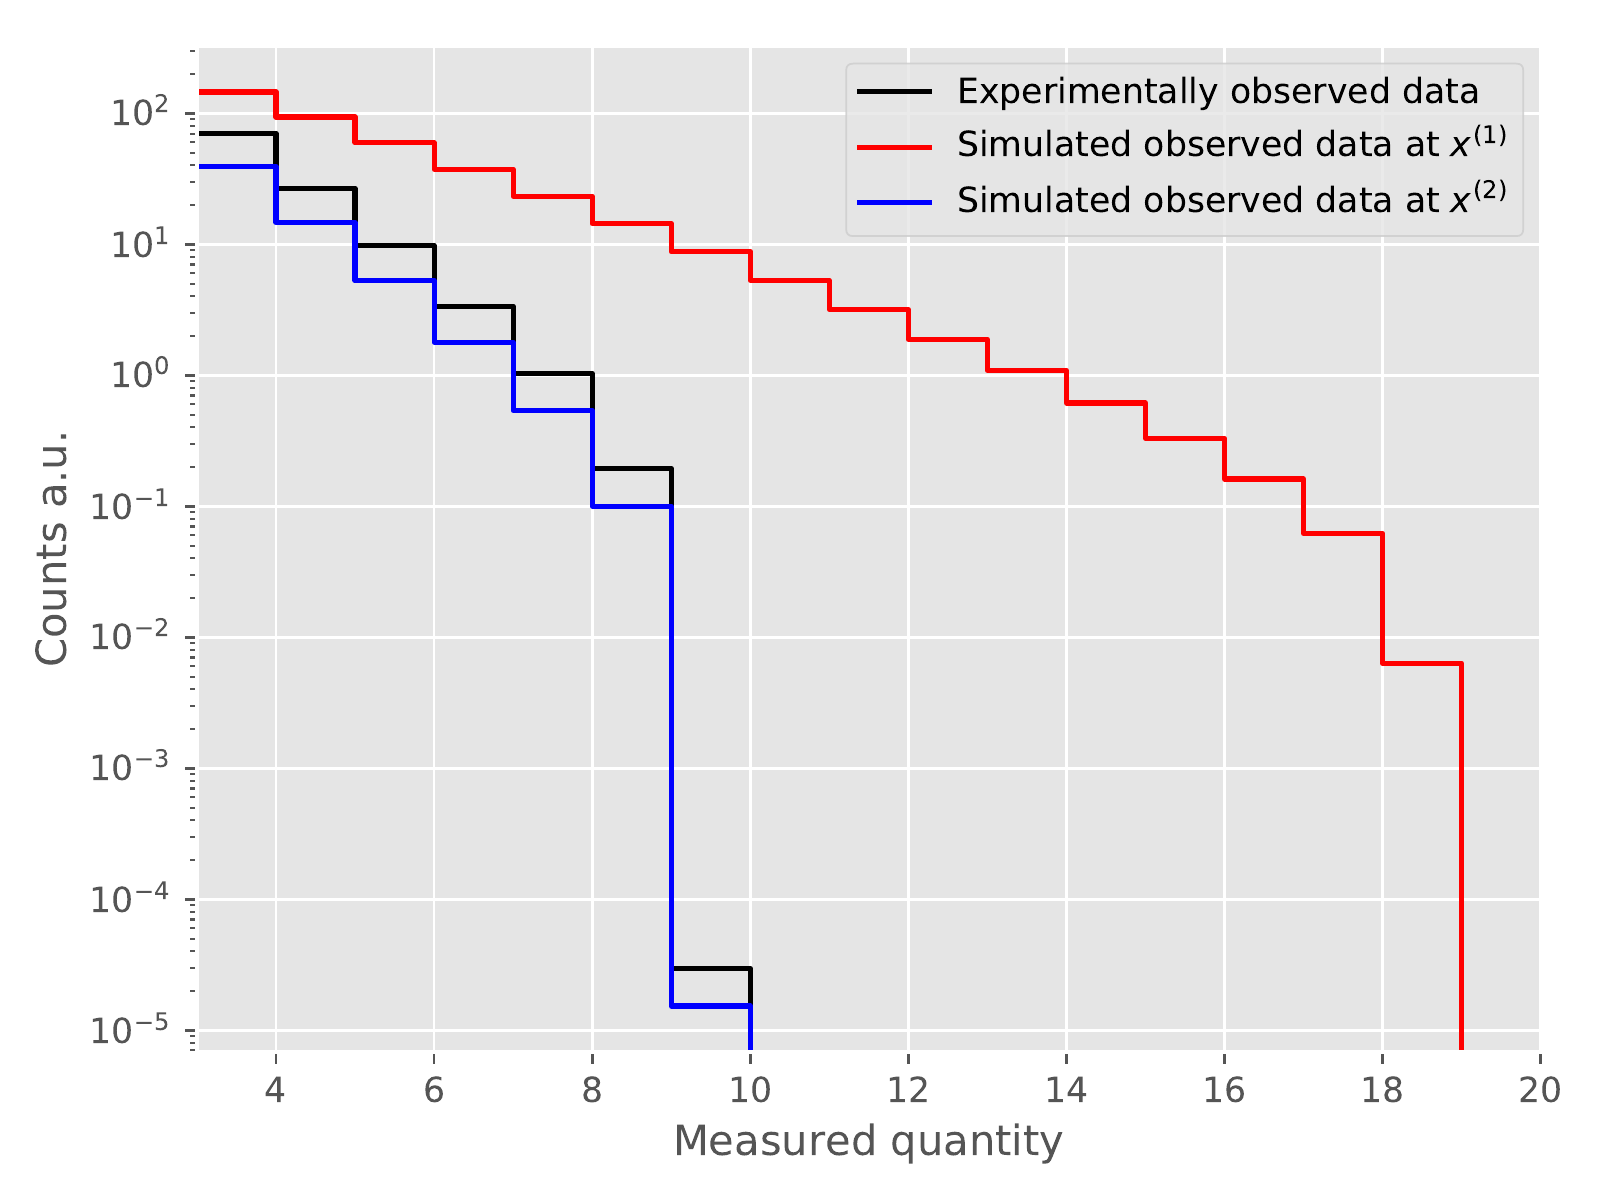}
%     \caption{\textcolor{blue}{Into supplement: Illustration of a typical problem setup in particle physics. Shown are
%         histogram skylines of observable experimental data (black) with observable
%         predictions coming from simulations at different points $x^{(k)}$ in the same parameter space (blue and red).
%         Numerical comparisons of the experimental with the simulated quantities are typically used to infer quantitative
%         statements on the (unobservable) parameters of the simulation. In this
%         example, one would e.g. be interested in finding parameter points $x$ such that the corresponding simulation
%        prediction resembles the experimental observation.}}
%     \label{fig:hepexample}
% \end{figure}

Our study consists of four separate analyses.    The first, or brute
force, analysis relies on the evaluation of $N_b(p^{(k)})$ over a dense set of 
parameter points $p^{(k)}$.   The second analysis uses a rational
approximation $r_b(p)$ based on far fewer parameter points.    A third
analysis is similar to the second, but demonstrates the effect of
poles.   The final analysis is based on a purely polynomial
approximation, similar to a previous study \cite{Cerdeno:2018bty}.
Our results are presented as 
two-dimensional projections of the 3-dimensional likelihood
called profile-likelihoods, which are quantities
normalised to the maximum observer likelihood.
These are produced using the tool superplot~\cite{Fowlie:2016hew}.
We have chose to show limits on the coupling strengths $c_+, c_\pi$
for a fixed value of $m_\chi$ \textcolor{blue}{(is the true?  if so, which value?).}

The results are summarized in Figure \cref{fig:nest-si-full} (fix this).
The darker regions in the plots represent a higher likelihood, or a
higher probability that the corresponding values of $c_+,c_\pi$ are
allowed by the data.
The top-left plot (\cref{fig:nest-si-full}) shows the projection of the likelihood obtained 
with  the full simulation \cref{eq:likelihood}.   
This is our ground truth for evaluating the approximation methods.
Qualitatively, we observe two ridges of equal likelihood in this
projection, showing that the allowed values of $c_+$ and $c_\pi$ are
highly correlated.   The top-right plot shows similar results using
the pole-free rational approximation, which is in good agreement with the ground truth both qualitatively
and quantitatively.   \textcolor{blue}{Is there a quantitative measure
  of the agreement between the projections?}
The bottom-left plot are the results using \cref{LinAlg},
which is less accurate due to spurious poles in the relevant parameter
domain.  Qualitatively, we find strong similarities with the ground truth, but the poles in some of the
$r_b(x)$ lead to a complete distortion of the evaluated likelihoods, and
therefore to a quantitatively wrong interpretation of the resulting plot as we
no longer find the dark region of equal likelihood present in
\cref{fig:nest-si-full,fig:nest-si-sip}.    Finally, the bottom-right
plot shows results using a polynomial approximation of order 7 (such that the number of coefficients is comparable to 
the number of coefficients used in the  rational approximations).  
The resulting likelihood projection \cref{fig:nest-si-poly} shows the
benefit of using rational approximations over polynomial ones; in this example,  the
polynomial approximations are  not able to capture the true likelihood
at all. 
Thus, the parameters inferred using the polynomial approximation would be misleading. 

The benefit of the rational approximation in our results is not simply
the agreement with the full simulation, but the relative computational
cost, summarized in \cref{tab:atimeloli}.
The algorithm terminates after about 30.000 evaluations of either $\mathcal{L}$ or the rational approximation
based $\tilde{\mathcal{L}}$. The difference in run-times is about a
factor of 50 to obtain similar results.   The number of parameters
considered in our case is modest, and we expect a significant speed-up
for likelihood evaluations using rational approximations for more
complex models.

\begin{table}
    \centering
    \begin{tabular}{l|c c}
        & Likelihood evaluations & total run-time~[s] \\ \hline
      using full simulation \cref{fig:nest-si-full} & 29459 & 14594 \\
    using $r_b$ with \cref{A:Polyak} & 29612 & 288
    \end{tabular}
    \caption{Summary of computational costs.}
    \label{tab:atimeloli}
\end{table}
