# Supplementary material for: Multivariate Rational Approximation
Source: arXiv:1912.02272 source file (2019-12-03)
Supplement: Supplementary file 3 [file studies-sm.tex]

%%%%%%%%%%%%%%%%%%%%%%%%%%%%%%%%%%%%%%%%%%%%%%%%%%%%%%%%%%%%%%%%%%%%%%%%
\section{Studies}

\begin{verbatim}
def coeffSolve2(self, VM, VN):
        """
        This does the solving for the numerator and denominator coefficients
        following Steve's recipe.
        """
        Feps = - (VN.T * self._Y).T
        # the full left side of the equation
        y = np.hstack([ VM, Feps[:,1:self._Y.size ] ])
        U, S, V = np.linalg.svd(y)
        # manipulations to solve for the coefficients
        # Given A = U Sigma VT, for A x = b, x = V Sigma^-1 UT b
        tmp1 = np.transpose( U ).dot( np.transpose( self._Y ))[0:S.size]
        Sinv = np.linalg.inv( np.diag(S) )
        x = np.transpose(V).dot( Sinv.dot(tmp1) )
        self._acoeff = x[0:self._M]
        self._bcoeff = np.concatenate([np.array([1.00]),x[self._M:self._M+self._N+1]])


\end{verbatim}

Define the rational polynomial approximation to $f(x)$ as $f(x) = p_M(x)/q_N(x)$ with $p_M(x) = a_0
+ a_1 x + \cdots + a_M x^M$ and $q_N(x) = 1 + b_1 x + \cdots + b_N
x^N$.
Note, in particular, that $b_0 \equiv 1$.
$f(x)$ is known at $K$ values of $x$ such that $f(x_i) \equiv f_i,
i=1,K$.   At any given point $x_i$, the coefficients of the
polynomials are constrained by the equation:
\begin{eqnarray*}
\begin{matrix}
p_M(x_i) - f(x_i) q_N(x_i) = 0 \\ 
a_0 + a_1 x_i + \cdots + a_M x_i^M - b_1 f_i  x_i - \cdots - b_N f_i x_i^N = f_i
\end{matrix}
\end{eqnarray*}
This manipulation is only possible if $b_0 \equiv 1$.

For $K$ such constraints, we have the matrix representation:

\newcommand{\MyMat}[3]{
                \begin{matrix}
                   \phantom{-}1 &  #1_1 & \cdots    & #1_1^{#2}\\ 
                   \phantom{-}1 & \cdots & \cdots   & \cdots\\
                   \phantom{-}1 &  #1_{#3} & \cdots & #1_{#3}^{#2} 
                \end{matrix}
}

\newcommand{\MyMatM}[3]{
                \begin{matrix}
                   -1 &  #1_1 & \cdots    & #1_1^{#2}\\ 
                   -1 & \cdots & \cdots   & \cdots\\
                   -1 &  #1_{#3} & \cdots & #1_{#3}^{#2} 
                \end{matrix}
}

\newcommand{\FMat}[4]{
                \begin{matrix}
                   #4_1 #1_1 & \cdots    & #4_1 #1_1^{#2}\\ 
                   \cdots & \cdots   & \cdots\\
                   #4_{#3} #1_{#3} & \cdots & #4_{#3} #1_{#3}^{#2} 
                \end{matrix}
}
\newcommand{\ColMat}{
a_0 \\
\cdots \\
a_M \\
b_1 \\
\cdots \\
b_N
}
\newcommand{\FColMat}{
f_1 \\
\cdots \\
\cdots \\
f_K
}

\newcommand{\spaceM}[1]{
\begin{matrix}
 \phantom{#1} \\
 \; \\
 \; \\ 
\end{matrix}
}

\begin{eqnarray*}
&
\begin{bmatrix}
\MyMat{x}{M}{K} \spaceM{1} 
\FMat{x}{N}{K}{-f}
\end{bmatrix}
\begin{bmatrix}
\ColMat
\end{bmatrix} 
= 
\begin{bmatrix}
\FColMat
\end{bmatrix} 
&\\
&\mathrm{or} &\\
&
\begin{bmatrix}
\bf M
\end{bmatrix}
\begin{bmatrix}
z
\end{bmatrix}
=
\begin{bmatrix}
c
\end{bmatrix}
&
\end{eqnarray*}

In particular, we are interested in those cases when $K > M + N$,
{\it{i.e.}} the problem is overconstrained.
%Our problem is in the form $ A x = b$, where $A$ is the matrix in the
%left of our equation, $x$ represents the coefficients of the
%polynomials, and $b$ represents the function values.   
An SVD decomposition of {\bf M}, given $c$, allows for a solution
of the coefficients $z$:
\begin{eqnarray*}
\begin{matrix}
M = U \Sigma V^T \\
z = V^T ( \Sigma^{-1} U^{T} c )\\
a_0 = z[0], a_1 = z[1], \cdots, a_M = z[M], b_0 = 1, b_1 = z[M+1], \cdots, b_N
= z[M+N]
\end{matrix}
\end{eqnarray*}

Our problem is ultimately one of minimization to
find the optimal polynomial coefficients given the constraints, which
are noisy in practice.    An alternative approach is to add the noise
from the start by shifting the function values $f_i$ by
$\pm\epsilon$ with the values $f_i^{\pm}$.    The constraints on the
coefficients are now doubled to $p(x_i)/q(x_i) < f_i^{+}$, and $f_i^{-}
< p(x_i)/q(x_i)$.

\renewcommand{\FColMat}[1]{
#1_1 \\
\cdots \\
\cdots \\
#1_K
}

\begin{eqnarray*}
\begin{bmatrix}
\MyMat{\phantom{-}x}{M}{K} \spaceM{1} \FMat{x}{N}{K}{-f^{+}} \\ 
\MyMatM{-x}{M}{K} \spaceM{1} \FMat{x}{N}{K}{\phantom{-}f^{-}}
\end{bmatrix} 
\begin{bmatrix}
\ColMat
\end{bmatrix}
<
\begin{bmatrix}
\FColMat{\phantom{-}b_0f^+} \\
\FColMat{-b_0f^-}
\end{bmatrix}
\end{eqnarray*}

This constraints problem is amenable to a  minimization
of the sum of squares of coefficients.
